# Supplementary material for: Parameter Estimation on Homogeneous Spaces
Source: arXiv:2411.00258 source file (2024-10-31)
Supplement: Supplementary file 1 [file applications.tex]

\documentclass[lettersize,journal]{IEEEtran}
\input{../../misc/preamble.tex}
\usepackage{tikz}
\usetikzlibrary{matrix, positioning, decorations.pathreplacing}

\begin{document}

\title{Applications of ``\textit{Parameter Estimation on Homogeneous Spaces}"}

\author{Shiraz Khan, Gregory S. Chirikjian,~\IEEEmembership{Fellow,~IEEE}%
\thanks{Corresponding email: \tt{shiraz@udel.edu}}%
% \thanks{Manuscript was drafted on August 28, 2024.}
}

\maketitle

% ----------------------------------------
\section{Localization using Relative Poses}
% In this section, we present the details of the sensor network localization problem considered in the main article.

% ----------------------------------------
\subsection{Sensor Network Model}
Let $(\mathcal V, \mathcal E)$ represent a graph with vertices $\mathcal V$ and edges $\mathcal E \subseteq \mathcal V \times \mathcal V$. The vertices are labeled as
$\mathcal V =\lbrace 1, 2, \ldots |\mathcal V|\rbrace$, where $|\,\cdot\,|$ denotes the cardinality of a set, and the edge connecting agents $i$ and $j$ is written as $(i,j)$. The pose of the $i^{th}$ agent is denoted by the $SE(2)$ transformation matrix $g_i$, which we will also write as $(\omega_i, \mf p_i)$, where $\omega_i \in \mathbb R$ is the agent's orientation and
$\mf p_i \in \mathbb R^2$ is the translation vector. Thus, we have the matrix representation of agent $i$'s pose:
\begin{align}
    g_i = \begin{bmatrix}
    \mf R(\omega_i) & \mf p\\
    \mf 0 & 1
    \end{bmatrix} \in SE(2)
\end{align}
where
\begin{align}
    \mf R(\omega) = \begin{bmatrix}
    \cos \omega & -\sin \omega\\
    \sin \omega & \cos \omega
    \end{bmatrix} \in SO(2).
\end{align}
The collective configuration of the sensor network is given by $g=(g_1, g_2, \ldots, g_{|\mathcal V|}) \in SE(2)^{|\mathcal V|}$.
% ----------------------------------------
\subsection{Measurement Model}
We assume that each agent is equipped with a camera (and possibly a range/depth sensor) that allows it to measure the relative pose of its neighbors. The relative pose between agents $i$ and $j$ is given by
\begin{align}
    g_i^{-1}g_j = \begin{bmatrix}
    \mf R(\omega_i)^\top \mf R(\omega_j) & \mf R(\omega_i)^\top (\mf p_j - \mf p_i)\\
    \mf 0 & 1
    \end{bmatrix} \in SE(2),
\end{align}
which is precisely the pose of agent $j$ as seen in agent $i$'s frame of reference. Note that agent $j$ sees the inverse of this matrix, i.e., $g_j^{-1}g_i = (g_i^{-1}g_j)^{-1}$. To simplify the presentation, we assume that each edge in $\mathcal E$ generates a single measurement. Thus, the sample space $\mathcal X$ is the space $SE(2)^{|\mathcal E|}$. A measurement $x\in \mathcal X$ is of the form $x = (x_{ij})$, where $i$ and $j$ range over the values satisfying $(i,j)\in \mathcal E$.

If the pose measurement is unimodal, and the measurements obtained at each edge is independent of the others, the measurements can be collectively modeled as an $SE(2)$ Gaussian distribution \cite{chirikjian2014gaussian}:
\begin{align}
    f(x|g) \propto \exp\left(-\frac{1}{2}\sum_{(i,j) \in \mathcal E} \lVert  \log\big((g_i^{-1}g_j)^{-1}x_{ij}\big) \rVert_{\mf S_{ij}}^2\right),
\end{align} 
where $\mf S_{ij}$ is a suitable positive definite weighting matrix which can capture the uncertainty in the measurement; for e.g., when camera images are used to measure the relative pose, there is typically more uncertainty along the depth direction than in the image plane. Note that $g_i^{-1}g_j$ represents the group-theoretic mean of the pose measurement $x_{ij}$.

It is readily observed that $g_i^{-1}g_j = (hg_i)^{-1}(hg_j)$.
This observation leads us to consider the following subgroup of $SE(2)^{|\mathcal V|}$, representing the group of symmetries with respect to which the measurement model is invariant:
\begin{align}
    H=\lbrace (h,h, \ldots,h) \, |\, h \in SE(2) \rbrace.
    \label{eq:subgroup}
\end{align}
Since the symmetry group acts from the left, we view the pose-based sensor network localization problem as a parameter estimation problem on $H \backslash SE(2)^{|\mathcal V|}$.

% \subsection{Gradient Computation}
% \red{TBD.}

% -------------------------------------------------------------------------
% -------------------------------------------------------------------------
%  *-*-*-*-*-*-*-*-*-*-  Distance Based Localization -*-*-*-*-*--*-*-*-*-* 
% -------------------------------------------------------------------------
% -------------------------------------------------------------------------

\section{Covariance Matrices}
Consider a zero-mean Gaussian distribution in $\mathbb R^n$ whose covariance is $\bm \Sigma \in \mathbb S(n)^{++}$ (the space of $d\times d$ positive definite matrices):
\begin{align}
    \bar f(\bm \Sigma) = \frac{1}{\sqrt{(2\pi)^n\det(\bm \Sigma)}}\exp\left(-\frac{1}{2}\mf x^\top_k \bm \Sigma^{-1} \mf x\right),
\end{align}
so that
\begin{align}
    \bar \ell (\bm \Sigma) &= -\frac{1}{2}\log\det(\bm \Sigma) - \frac{1}{2}\mf x^\top \bm \Sigma^{-1} \mf x + \textrm{const}\\
    &=  - \frac{1}{2}\log\det(\bm \Sigma) -\frac{1}{2}\tr(\bm \Sigma^{-1}\mf X) + \textrm{const}.
\end{align}
where $\mf X \coloneqq \mf x\mf x^\top$.

As mentioned in the paper, we can identify $\mathbb S(n)^{++}$ with the space $GL(n)^+/SO(n)$. The Lie algebra $\mathfrak h=\mathfrak{so}(n)$ consists of skew-symmetric matrices, so a natural choice of $\mf m$ is the space $\mathbb S(n)$ of symmetric matrices. Conveniently, $\mathfrak h$ and $\mf m$ are orthogonal with respect to the Frobenius inner product for $GL(n)^+$, which is given by $\langle A, B\rangle = \tr(A^\top B)$. Since any matrix $\mf A \in \mathfrak{gl}(n)^+$ can be decomposed as 
\begin{align}
    \mf A = \frac{1}{2}(\mf A + \mf A^\top) + \frac{1}{2}(\mf A - \mf A^\top),
\end{align}
this indeed represents a reductive decomposition of $\mathfrak{gl}(n)^+$ into $\mathfrak h \oplus \mf m$.

To apply our theory, we need to rewrite the statistical model so that it has the required invariance, $\ell(g) = \ell(g h)$. One way of doing this is to consider
\begin{align}
    \ell (g) &=   - \frac{1}{2}\log\det((g g^\top)^{-1}) -\frac{1}{2}\tr((g g^\top)^{-1}\mf X) + \textrm{const}.
\end{align}
as the pullback statistical model on $GL(n)^+$,
where $g \in GL(n)^+$. Here, $g$ represents the transformation $\mf x \mapsto g \mf x$ which makes the vector $g \mf x$ a standard Gaussian.

\section{Derivatives}
To compute the gradient of $\ell$ with respect to $\bm \Sigma$, we can exploit the following characterization of the gradient (where we let ${\rm grad} \ell (\bm \Sigma) \coloneq {\bf grad} \ell (\bm \Sigma)^\wedge$):
\begin{align}
    \langle {\rm grad} \ell (\bm \Sigma), Z\rangle = Z^L \ell(\bm \Sigma).
\end{align}
We have,
\begin{align}
    \tr({\rm grad} \ell (\bm \Sigma)^\top Z) &= \frac{d}{dt} \ell(\bm \Sigma \exp(tZ))\big|_{t=0} \\
    &= -\frac{1}{2}\frac{d}{dt}\log\det(\bm \Sigma + t\bm \Sigma Z)\Big|_{t=0} \nonumber\\
    &\quad - \frac{1}{2} \frac{d}{dt}\tr((\mf I - t Z)\bm \Sigma^{-1} \mf X)\Big|_{t=0}
\end{align}
Using the calculation in \cite[p. 641]{boyd2004convex} for the first term, we get\footnote{We have explicitly written the transpose $(\,\cdot\,)^\top$ of $\bm \Sigma$ despite it being a symmetric matrix. This is because we should view $f$ as the pullback statistical model on $GL(n)^+$ in order to apply our theory.}
\begin{align}
    \tr({\rm grad} \ell (\bm \Sigma)^\top Z) &= -\frac{1}{2}\tr(Z)  + \frac{1}{2}\tr(Z\bm \Sigma^{-1} \mf X),
\end{align}
meaning that 
\begin{align}
    {\rm grad} \ell (\bm \Sigma) &= \frac{1}{2} \left(\mf X{\bm \Sigma^{-1}}^\top - \mf I \right),
\end{align}
Finally, we should project the gradient vector onto $\mf m$, which is done using $\mf A \mapsto \frac{1}{2}(\mf A + \mf A^\top)$, as follows:
\begin{align}
    \overline{\rm grad} \ell (\bm \Sigma) &= \frac{1}{4} \left(\mf X{\bm \Sigma^{-1}}^\top + \bm \Sigma^{-1}\mf X - 2\mf I \right).
    % &= \frac{1}{4} \left((\mf X - \bm \Sigma)\bm \Sigma^{-1} + \bm \Sigma^{-1}(\mf X- \bm \Sigma)  \right).
\end{align}

\subsection{Computing the {\bf FIM}}
Using superscripts to represent components of matrices and vectors and $\mf S\coloneqq {\bm \Sigma}^{-1}$, we have,
\begin{align}
    (\bm \Sigma^{-1}\mf X)^{ij} = \mf S^{ik}\mf x^k \mf x^j
\end{align}
and
\begin{align}
    \overline{\rm grad} \ell (\bm \Sigma)^{ij} &= \frac{1}{4} \left(\mf S^{ik}\mf x^k \mf x^j + \mf S^{jk}\mf x^k \mf x^i - 2\delta_{ij} \right).
\end{align}

To compute the ${\bf FIM}$, we can use the fact that
\begin{align}
    \overline {\mf F}_g = \mathbb E \left[\overline{\bf grad} \ell (\bm \Sigma)  \overline{\bf grad} \ell (\bm \Sigma)^\top\right].
\end{align}
\bibliographystyle{IEEEtran}
\bibliography{../../references}
\end{document}
